# Supplementary material for: Nucleon-nucleon correlation functions from different interactions in comparison
Source: arXiv:2505.13433 ancillary file (2025-05-19)
Supplement: Supplementary file 1 [file nn_cf_supp_mat.pdf]

# Supplementary material for
# "Nucleon-nucleon correlation functions from different interactions in comparison"

Matthias Göbel [a], Alejandro Kievsky [a]

[a] *Istituto Nazionale di Fisica Nucleare, Sezione di Pisa, Largo Pontecorvo 3, 56127 Pisa, Italy*

19.05.2025

**Abstract**

We provide supplementary figures regarding the composition of the *pp* correlation function, the convergence of the correlation functions in the included channels, and on the influence of the coupling between channels. Moreover, this material contains detailed data regarding the partial-wave truncation and numerical uncertainties of the correlation functions and of the sensitivity curves.

## 1. Supplementary figures

### *1.1. Composition of the pp correlation function*

In Fig. 1, the fraction of the *pp* correlation function with a certain $l_{\text{max,int}}$ ($l_{\text{max,free}} = l_{\text{max,int}}$) in regards to the overall *pp* correlation in percent is shown in order to give a quantitative and easy-to-read-off impression of the composition of the correlation function.

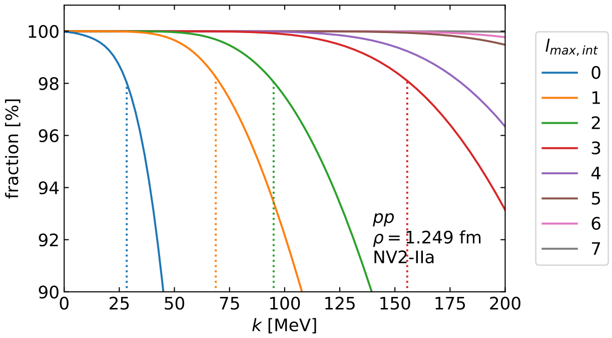


Figure 1: The plots shows the fraction of a *pp* correlation function obtained with the $l_{\text{max,int}}$ given in the legend in relation to the *pp* correlation function obtained with $l_{\text{max,int}} = 10$ and $l_{\text{max,free}} = 35$. The NV2-IIa interaction is used. The dotted vertical lines indicate the momenta at which the fraction goes below 98 %.

### *1.2. Convergence in the included channels*

Figure 2 depicts the deviation of correlation functions obtained with different $j_{\text{max,int}}$ from a reference correlation function. This supplements Fig. 7 of the paper itself by displaying not only the *pp* case but also the *nn* and *np* cases.

*Email addresses:* `matthias.goebel@pi.infn.it` (Matthias Göbel), `alejandro.kievsky@pi.infn.it` (Alejandro Kievsky)

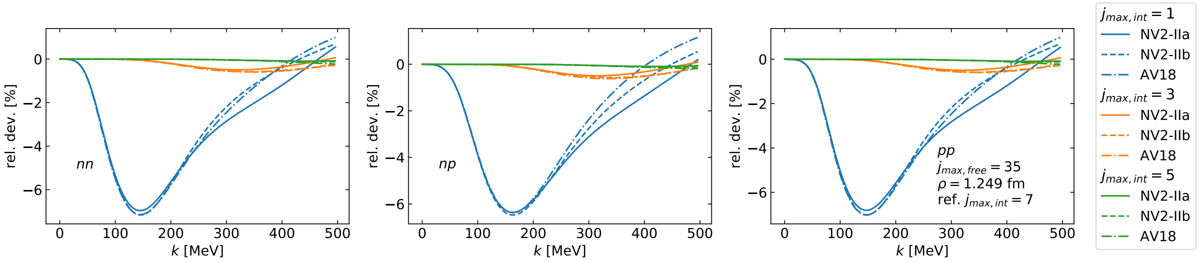


Figure 2: The relative deviation of correlation functions obtained at different $j_{\mathrm{max,int}}$ from the corresponding correlation function obtained with $j_{\mathrm{max,int}} = 7$ is shown. The line styles encode the underlying interaction. The left panel depicts *nn* correlation functions, the middle one depicts *np* correlations, and the right one shows the *pp* ones.

### *1.3. Influence of the coupling of channels*

In supplementation to subsection "3.5. Influence of the coupling of channels" of the paper itself, Fig. 3 displays the relative deviations between correlation functions obtained with no coupling between different partial waves and those with coupling taken into account.

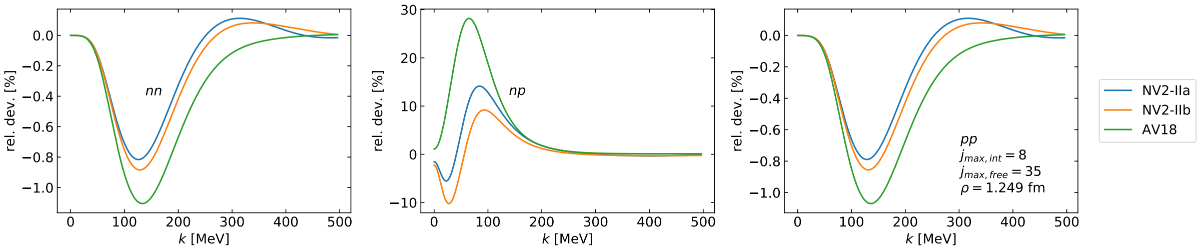


Figure 3: The relative deviation of correlation functions with no coupling between different partial-wave channels and the corresponding one with coupling included is shown. The different colors encode the employed interaction, while the panels differ in the considered system (from left to right: *nn*, *np*, and *pp*).

## 2. Uncertainty estimates for the results

In this section, we provide some data and details on the accuracy of our results for correlation functions and their relative deviations in regards to variation of truncation parameters and solving the underlying ODE.

### *2.1. Uncertainties of correlation functions*

Here we investigate how accurate the results for the correlation functions reported in Fig. 4 of the paper are. For that purpose we look at the relative deviations between the correlation functions stemming from a variation of the truncation in the free partial waves given by $j_{\mathrm{max,free}}$, a variation of the truncation in the interacting partial waves given by $j_{\mathrm{max,int}}$, and the variation of the adaptive ODE solver's accuracy goal and maximum step width. The results are depicted for the example of the *np* correlation function in Fig. 4.

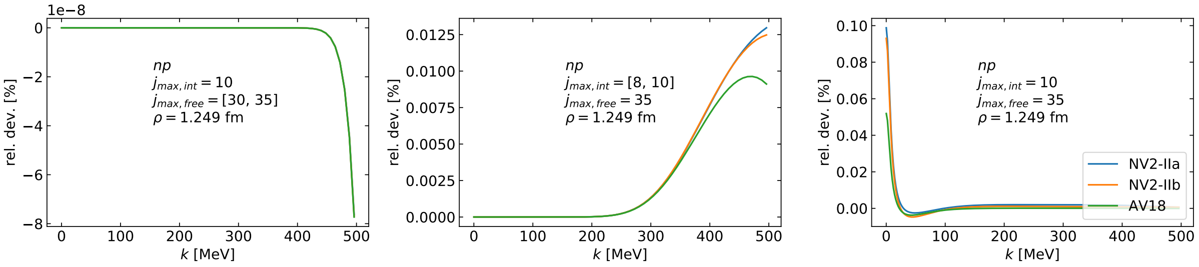


Figure 4: Estimates for the relative uncertainties (in percent) of the $np$ correlation function. In the left panel, the truncation parameter $j_{\text{max,free}}$ is varied, while in the middle panel it is $j_{\text{max,int}}$. The right panel is based on a variation of the adaptive ODE solver's settings.

We see that the uncertainties are well under control. Naturally, the uncertainties due to the truncation in free and interacting partial waves rise towards higher momenta, as the higher partial waves become more important in that region. In the low-momentum region, the dominant source of uncertainties is the ODE solver. The qualitative behavior of the $nn$ relative uncertainties are very similar and the orders of magnitude associated with these three different uncertainty types are also the same for the $nn$ system. Based on this plot and on the same studies for the other systems, we conclude that the uncertainty is in general below 0.2 %. We conclude that the results for the correlations are well converged.

### 2.2. *Uncertainties of relative deviations*

In this part, we investigate how accurate the results for the relative deviations between the correlation functions reported in Fig. 8 of the paper are. We vary the same parameters and settings as in the previous subsection: $j_{\text{max,free}}$, $j_{\text{max,free}}$, and ODE solver settings. The results are depicted in Fig. 5 for the example of relative deviations between the $pp$ correlation functions of different interactions.

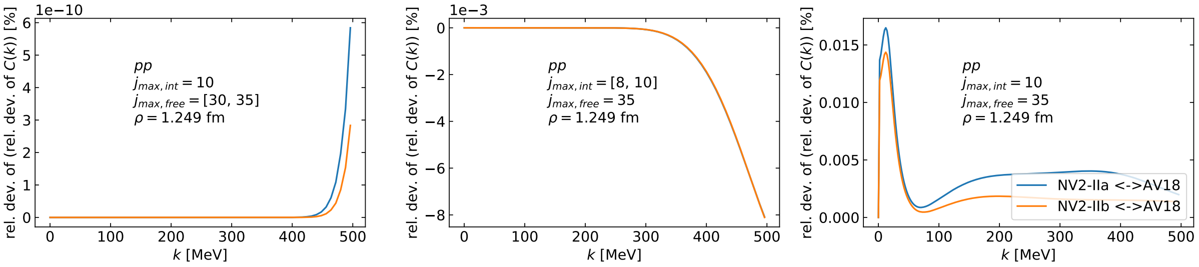


Figure 5: Estimates for the relative uncertainties (in percent) of the $pp$ correlation function's sensitivity to interactions. In the left panel, the truncation parameter $j_{\text{max,free}}$ is varied, while in the middle panel it is $j_{\text{max,int}}$. The right panel is based on a variation of the adaptive ODE solver's settings.

As expected, the general pattern here is similar as in the previous subsection. Our investigations show that the same plot for the $nn$ and for the $np$ system look similar. The most notable difference is that the uncertainty due to the ODE solving does not vanish at $k = 0$ but peaks there for the $nn$ and the $np$ system, as in those systems the correlation function is finite at zero momentum. Based on these results for all three systems, we estimate that the overall uncertainties in terms of relative percentages for our relative deviation results are below 0.1 %. In other words uncertainties of the percentages reported in Fig. 8 of the paper are below a thousandth part of the percentages. The results for the relative deviations between the correlation functions are well converged.
